# Supplementary material for: Computational Challenges in Non-parametric Prediction of Bradycardia in Preterm Infants
Source: arXiv:2011.09307 source file (2020-11-17)
Supplement: Supplementary file 1 [file appendix1.tex]

\chapter{List of Acronyms}
\begin{acronym}
\acro{1D}{one-dimensional}
\acro{2D}{two-dimensional}
\acro{ADC}{analog-to-digital converter}
\acro{AWGN}{additive white Gaussian noise}
\acro{BEC}{bounding exponential chirp}
\acro{BFP}{bootstrap particle filter}
\acro{CDM}{code division multiplexing}
\acro{CDMA}{code division multiple access}
\acro{CFAR}{constant false alarm rate}
\acro{CIR}{constant information radar}
\acro{CP-FM}{cubic polynomial FM}
\acro{CPI}{coherent processing interval}
\acro{CRLB}{Cram\'{e}r-Rao lower bound}
\acro{CSS}{chirped spread spectrum}
\acro{DARPA}{The Defense Advanced Research Projects Agency}
\acro{DE}{differential evolution}
\acro{DSSS}{direct-sequence spread spectrum}
\acro{ELINT}{electronic intelligence}
\acro{EO}{electro-optical}
\acro{FDOA}{frequency difference of arrival}
\acro{FIM}{Fisher information matrix}
\acro{FM}{frequency-modulated}
\acro{FMCW}{frequency-modulated continuous-wave}
\acroplural{GMM}[GMMs]{Gaussian mixture models}
\acro{GMM}{Gaussian mixture model}
\acro{GPS}{Global Positioning System}
\acro{GSM}{Global System for Mobile Communications}
\acroplural{IF}[IFs]{instantaneous frequencies}
\acro{IF}{instantaneous frequency}
\acro{ISB}{isolated sub-band}
\acro{ITS}{intelligent transportation systems}
\acro{LTE}{Long-Term Evolution}
\acro{MAC}{multiple access channel}
\acro{MIMO}{multiple-input multiple-output}
\acro{MLE}{maximum likelihood estimator}
\acro{MMSE}{minimum mean-squared error}
\acro{MSE}{mean-squared error}
\acro{MTI}{moving target indicator}
\acro{MUDR}{multiuser detection radar}
\acro{OFDM}{orthogonal frequency-division multiplexing}
\acro{PAPR}{peak-to-average power ratio}
\acro{PDA}{probabilistic data association}
\acro{PF}{particle filter}
\acro{PMSE}{predicted \ac{MSE}}
\acro{PPM}{pulse-position modulation}
\acro{PRF}{pulse repetition frequency}
\acro{PRI}{pulse repetition interval}
\acro{PSP}{principle of stationary phase}
\acro{QPC}{quadratic parabolic chirp}
\acro{QPPF}{quartic polynomial phase function}
\acro{RFID}{radio-frequency identification}
\acro{RMS}{root mean square}
\acro{SDR}{software-defined radio}
\acro{SDT}{scaled-difference transform}
\acro{SFM}{sawtooth \ac{FM}}
\acro{SIC}{successive interference cancellation}
\acro{SNR}{signal-to-noise ratio}
\acro{SSPARC}{shared spectrum access for radar and communications}
\acro{SRI}{sweep repetition interval}
\acro{STAP}{space-time adaptive processing}
\acro{TB}{time-bandwidth}
\acro{TBD}{track-before-detect}
\acro{TDM}{time-division multiplexing}
\acro{TFM}{triangular \ac{FM}}
\acro{UKF}{unscented Kalman filter}
\acro{UMTS}{Universal Mobile Telecommunications System}
\acro{UPF}{unscented particle filter}
\acro{UT}{unscented transform}
\acro{V2V}{vehicle-to-vehicle}
\acro{WF}{water-filling}
\end{acronym}
